# Supplementary material for: Can Knowledge of End-to-End Text-to-Speech Models Improve Neural MIDI-to-Audio Synthesis Systems?
Source: arXiv:2211.13868 source file (2023-03-21)
Supplement: Supplementary file 1 [file appendix.tex]

\newpage
\clearpage
\appendix
\onecolumn
\section{Appendix}

We provide additional details on experiments, including MOS distribution and rainbow-gram.

\begin{figure*}[h]
    \centering
    \includegraphics[scale=0.8]{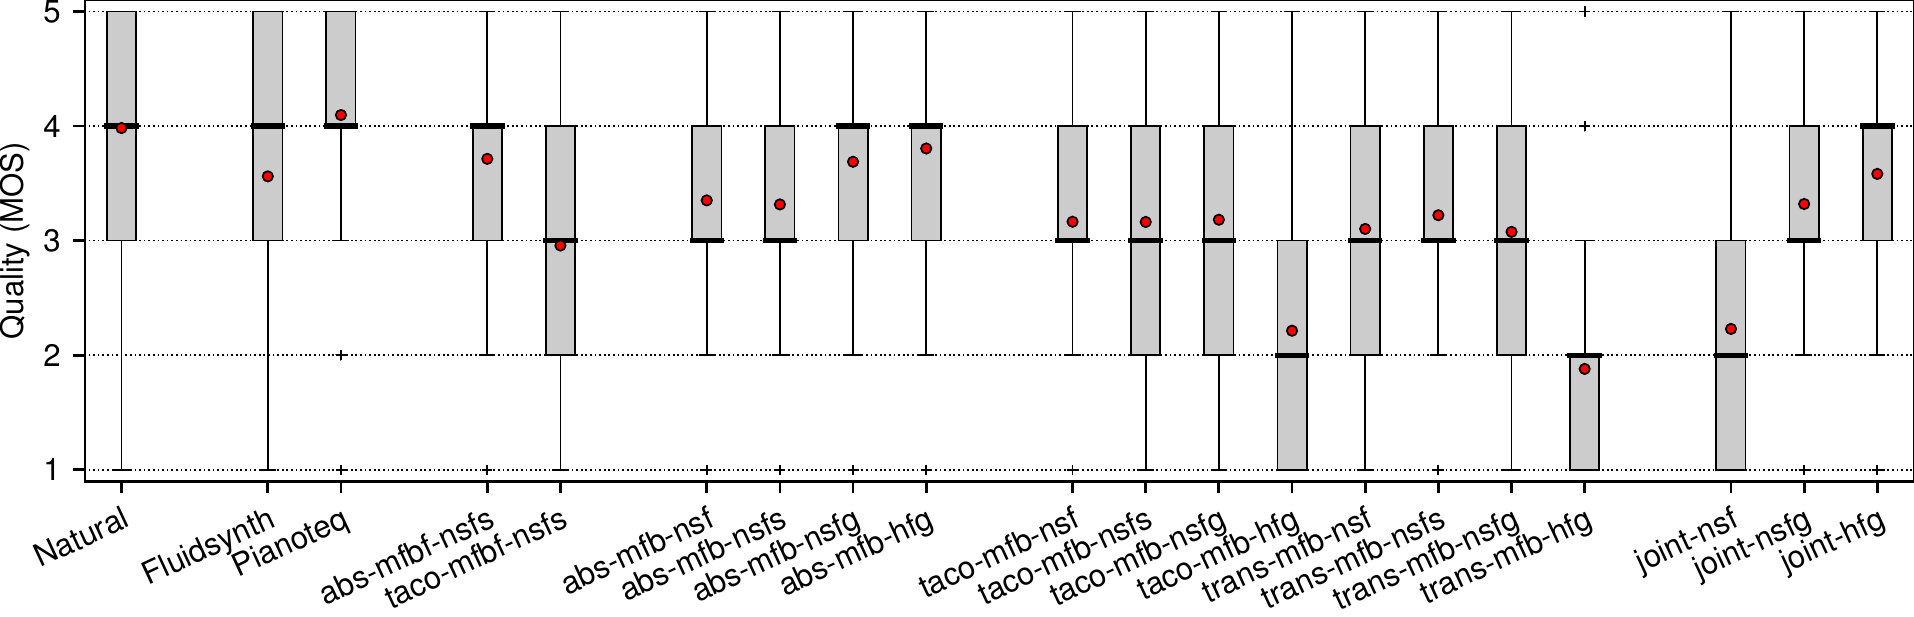}
    \caption{Boxplots of MOS per system. Red dots denote mean of MOS.}
    \label{fig:maestro_box}
\end{figure*}

\begin{figure*}[h]
    \centering
    \includegraphics[scale=0.83]{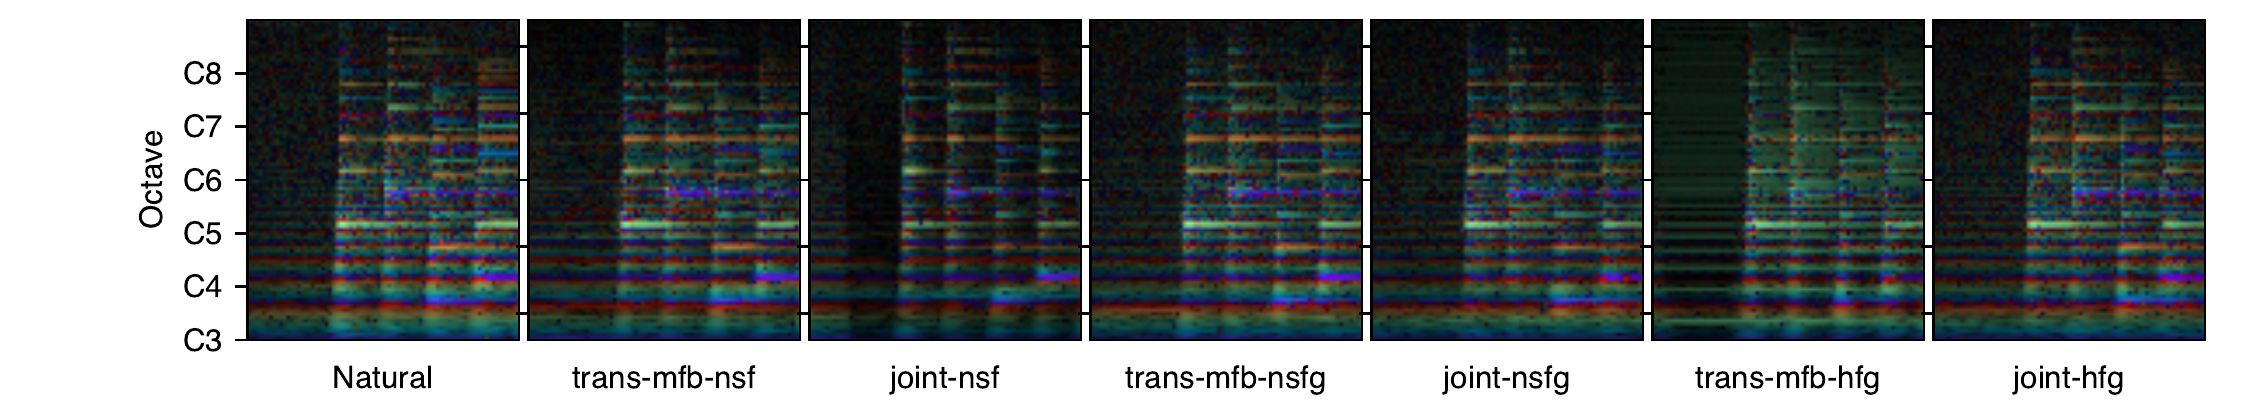}
    \caption{Rainbow-grams of audio samples from selected systems.}
    \label{fig:my_label}
\end{figure*}
